# Supplementary material for: On the Dual-Phase-Lag thermal response in the Pulsed Photoacoustic effect: 1D approach
Source: arXiv:2406.13852 source file (2024-07-09)
Supplement: Supplementary file 1 [file Suplemental_material.tex]

% ****** Start of file aipsamp.tex ******
%
%   This file is part of the AIP files in the AIP distribution for REVTeX 4.
%   Version 4.1 of REVTeX, October 2009
%
%   Copyright (c) 2009 American Institute of Physics.
%
%   See the AIP README file for restrictions and more information.
%
% TeX'ing this file requires that you have AMS-LaTeX 2.0 installed
% as well as the rest of the prerequisites for REVTeX 4.1
% 
% It also requires running BibTeX. The commands are as follows:
%
%  1)  latex  aipsamp
%  2)  bibtex aipsamp
%  3)  latex  aipsamp
%  4)  latex  aipsamp
%
% Use this file as a source of example code for your aip document.
% Use the file aiptemplate.tex as a template for your document.

\documentclass[%
 aip,
%jmp,
% bmf,
% sd,
% rsi,
amsmath,amssymb,
preprint,%
%reprint,%
%author-year,%
%author-numerical,%
% Conference Proceedings
]{revtex4-1}

\usepackage{tabularx}
\usepackage[english]{babel}
\usepackage[utf8]{inputenc}
\usepackage[T1]{fontenc}
\usepackage{textcomp}
\usepackage{float}
\usepackage{amssymb,amsbsy} 
\usepackage{amsmath}
\usepackage{verbatim}
\usepackage{subfigure}
\usepackage{hyperref}
\usepackage{xcolor}
\usepackage{soul}
\usepackage{cleveref}
\usepackage{ragged2e}
\usepackage{fbox}
%\linenumbers
\usepackage{graphicx}% Include figure files
\usepackage{dcolumn}% Align table columns on decimal point
\usepackage{bm}% bold math
\setlength\parindent{0pt}
\usepackage{dcolumn}
\usepackage{hyperref}% add hypertext capabilities
\usepackage[mathlines]{lineno}% Enable numbering of text and display math
%\linenumbers\relax % Commence numbering lines

\begin{document}

%\begin{linenumbers}

%\begin{frontmatter}

\title{Supplemental material: On the Dual-Phase-Lag thermal response in the Pulsed Photoacoustic effect: a theoretical and experimental 1D-approach}

\author{L. F. Escamilla-Herrera}%\email{lescamilla@fisica.ugto.mx}
\affiliation{Divisi\'on de Ciencias e Ingenier\'ias Campus Le\'on, Universidad de Guanajuato, A.P. E-143, C.P. 37150, Le\'on, Guanajuato, M\'exico.}
\author{J.M. Derramadero-Domínguez}%\email{marioderramadero@gmail.com}
\affiliation{Departamento de Ingeniería Mecatrónica, Tecnológico Nacional de México / Instituto Tecnológico de Celaya, Av. Antonio García Cubas 600, Celaya, Gto., 38010, México.}
\author{O. M. Medina-Cázares} %\email{om.medina@ugto.mx}
\affiliation{Divisi\'on de Ciencias e Ingenier\'ias Campus Le\'on, Universidad de Guanajuato, A.P. E-143, C.P. 37150, Le\'on, Guanajuato, M\'exico.}
\author{J. E. Alba-Rosales}%\email{aubeq@cio.mx}
\affiliation{Centro de Investigaciones en Óptica AC, Loma del Bosque 115, CP 37150, León, GTO., México.}
\author{F.J. García-Rodríguez} %\email{}
\affiliation{Departamento de Ingeniería Mecatrónica, Tecnológico Nacional de México / Instituto Tecnológico de Celaya, Av. Antonio García Cubas 600, Celaya, Gto., 38010, México.}
\author{G. Gutiérrez-Juárez}\email{ggutj@fisica.ugto.mx}
\affiliation{Divisi\'on de Ciencias e Ingenier\'ias Campus Le\'on, Universidad de Guanajuato, A.P. E-143, C.P. 37150, Le\'on, Guanajuato, M\'exico.}

\date{\today}% It is always \today, today,
             %  but any date may be explicitly specified
             
\maketitle

%\begin{keyword}
%Stress confinement, 1D-heat diffusion equation, Dual-Phase-Lag, Laser-induced ultrasound.
%\end{keyword}

%\end{frontmatter}

\begin{widetext}

\section{Photothermal boundary conditions in time domain}

\begin{table}[h]
    \centering
    \begin{tabular}{c}
        Temperature BC \\
        \hline
        $T_{B}(z,t)\big|_{z=0} = T_{S}(z,t)\big|_{z=0}$   \\
        $T_{S}(z,t)\big|_{z=L} = T_{F}(z,t)\big|_{z=L}$ \\
        $\kappa_{l} \left(\frac{\partial }{\partial z}T_{B}(z,t)\right)\big|_{z=0} = \kappa_{s} \left(\frac{\partial }{\partial z}T_{S}(z,t)\right)\big|_{z=0}$  \\
        $\kappa_{s} \left(\frac{\partial }{\partial z}T_{S}(z,t)\right)\big|_{z=L} = \kappa_{l} \left(\frac{\partial}{\partial z} T_{F}(z,t)\right)\big|_{z=L}$   \\
          \\
        Pressure BC  \\
        \hline
        $P_{B}(z,t)\big|_{z=0} = P_{S}(z,t)\big|_{z=0}$  \\
        $P_{S}(z,t)\big|_{z=L} = P_{F}(z,t)\big|_{z=L}$ \\
        $\frac{1}{\rho_l} \left(\frac{\partial }{\partial z}P_{B}(z,t)\right)\big|_{z=0} = \frac{1}{\rho_{s}} \left(\frac{\partial}{\partial z} P_{S}(z,t)\right)\big|_{z=0}$  \\
        $\frac{1}{\rho_s} \left(\frac{\partial }{\partial z}P_{S}(z,t)\right)\big|_{z=L} = \frac{1}{\rho_l} \left(\frac{\partial }{\partial z}P_{F}(z,t)\right)\big|_{z=L}$  \\
    \end{tabular}
    \caption{Photo-thermal boundary conditions for temperature and pressure in the time domain for the 1D three-layer problem. \label{boundary}}
    \label{tab:my_label}
\end{table}

\section{Thermal solution coefficients}

\begin{subequations}\label{T_coef}
\begin{align}
  a_{1B} &= a_{1S} + a_{2S} + \hat{T}_{0}; \\
  a_{2B} &= 0;\\
  a_{1S} &= - \frac{e^{-L\mu}(\Lambda+1)(\epsilon\Lambda-1) + e^{- L \sigma_s}(\Lambda-1)(\epsilon\Lambda+1)}{(\Lambda+1)^2-e^{-2L\sigma_s}(\Lambda-1)^2}  e^{-L\sigma_s}\hat{T}_{0}; \\
  a_{2S} &= -e^{-L(\mu-\sigma_s)}  \frac{\left(-(\Lambda-1)(\epsilon\Lambda-1) + e^{L(\mu + \sigma_s)}(\Lambda+1)(\epsilon\Lambda+1)\right)}{-(\Lambda-1)^2 + e^{2L\sigma_s}(\Lambda+1)^2} \hat{T}_{0};\\
  a_{1F} &= 0; \\
  a_{2F} &=  e^{\sigma_l L}\left( a_{1S} e^{\sigma_s L} + a_{2S} e^{-\sigma_s L} + \hat{T}_{0} e^{-\mu L} \right)\,.
\end{align}
\end{subequations}

Where we have defined two auxiliary functions, namely, $\Lambda(\omega;\tau_{_T}) = \kappa_s \sigma_s/\kappa_l \sigma_l$ and $\epsilon(\omega;\tau_{_T}) = \mu/\sigma_s$. 

\section{Pressure solution coefficients}

\begin{subequations}\label{P_Coef}
\begin{align}
  b_{1B} &= b_{1S} + b_{2S} - \hat{P}_{T_B} + \hat{P}_{T_S}; \\
  b_{2B} &= 0; \\
  b_{1S} &= \left[ \frac{\hat{P}_{T_S} - \hat{P}_{T_B}}{\gamma + 1} + \frac{i}{k_{l}}\frac{\rho_{l} \hat{P}'_{T_S} - \sigma_{l}\hat{P}_{T_B}}{ \gamma + 1} - \frac{e^{i k_{s} L}}{k_{l}}\frac{ i \rho_{l} \hat{P}'_{T_S}}{ \gamma -1} \right]\left(\frac{\gamma -1}{\gamma + 1} - e^{i 2 k_s L} \ \frac{\gamma + 1}{\gamma - 1}\right)^{-1}; \\
  b_{2S} &= -\frac{\hat{P}_{T_S} - \hat{P}_{T_B}}{\gamma + 1} + b_{1S} \frac{\gamma -1}{\gamma + 1} -  \frac{i}{k_{l}}\frac{\rho_{l} \hat{P}'_{T_S} - \sigma_{l}\hat{P}_{T_B}}{ \gamma + 1};\\
  b_{1F} &= 0;\\
  b_{2F} &= e^{i k_{l} L} \left(b_{1S} \ e^{i k_{s} L} + b_{2S} \ e^{-i k_{s} L} + \hat{P}_{T_S}\right)\,.
\end{align}
\end{subequations}

Where we have defined the auxiliary function,
\begin{displaymath}
    \gamma(\omega) = \frac{\rho_l k_s}{\rho_s k_l} = \frac{Z_l}{Z_s}\,;
\end{displaymath}
and the normalized first-order derivative of $\hat{P}_{T_S}(\omega; \tau_{_T})$ with respect to $z$, 
\begin{displaymath}
    \hat{P}'_{T_S}(z,\omega;\tau_{_T}) = \frac{1}{\rho_s}\frac{\partial}{\partial z} \hat{P}_{T_S} =  - e^{-z (\mu + \sigma_s)} \omega^2 \beta_s \left[ \frac{ \sigma_s a_{2S}(\omega;\tau_{T})}{k_s^2 + \sigma_s^2}e^{\mu z} + \frac{\mu \hat{T}_{0}(\omega;\tau_{_T})}{k_s^2 + \mu^2} e^{\sigma_s z} \right]\,.
\end{displaymath}
Here $Z_j$ is the characteristic impedance of the corresponding medium.

\subsection{Thermomechanical properties for numerical calculations}

\begin{table}[h]
    \centering
    \begin{tabular}{c | c | c | c | c}
    \textbf{Physical constant}  & \textbf{Symbol} & \textbf{Units} (in MKS) & \textbf{Water}  & \textbf{Aluminum} \\   
    \hline
    \hline
    Thermal conductivity   & $\kappa$ & $W/m \ K$ & 0.6  & 237\\
    Density    & $\rho$ & $Kg/m^3$ & 1000 & 2700 \\
    Thermal diffusivity  & $\chi$ & $m^2/s$ & $1.43 \times 10^{-7}$ & $9.79\times 10^{-5}$\\
    Volumetric expansion  & $\beta$  & $K^{-1}$ & $2.07\times 10^{-4}$ & $7\times 10^{-5}$\\
    Speed of sound  & $c$ & $m/s$ & 1593 & 6400 \\
    Specific heat at constant pressure  & $C_P$ & $J/Kg K$ & $4.18\times10^3$ & 896 \\
    Compressibility modulus & $K_f$ & $Pa$ & $2.2\times 10^9$ & DNA\\
    Young’s modulus & $a$  & $Pa$ & DNA & $6.9\times 10^{10}$ \\
    Isothermal compressibility  & $\kappa_{_T}$  & $Pa^{-1}$ & $5\times 10^{-10}$ & $1.4\times 10^{-11}$\\
    Optical absorption coefficient (for 532 nm) & $\mu$ & $m^{-1}$ & 0.12 & $1.5156\times 10^6$ \\
    \hline
    \end{tabular}
    \caption{Values of the thermomechanical properties considered for the numerical calculations presented in the main manuscript (DNA stands for "does not apply").}
    \label{tab:table2}
\end{table}

\end{widetext}

%\newpage

%\end{linenumbers}

\end{document}
